# Supplementary material for: Formal Specification and Verification of Smart Contracts for Azure Blockchain
Source: arXiv:1812.08829 source file (2019-04-29)
Supplement: Supplementary file 1 [file appendix.tex]

\begin{appendix}
\section{Runtime Checking for Semantic Conformance}
\label{sec:runtime-checks}
We briefly discuss some choices for realizing runtime checks in the presence of a non-deterministic function such as $\SolidityNonDetFn$.
We do this by essentially eliminating (quantifying out) $\SolidityNonDetFn$ from any expression it appears in.
Consider a predicate $\phi$ containing a call to $\SolidityNonDetFn$ that appears in either \texttt{require} or \texttt{assert} as part of the instrumentation described above; further let $\phi$ contains $k$ calls to $\SolidityNonDetFn{}$.
We have two such options:
\begin{enumerate}
\item Replace $\phi$ with $\phi_0 \wedge \ldots \phi_{2^k - 1}$, where $\phi_i$ replaces the vector of calls to $\SolidityNonDetFn{}$ with the Boolean vector for the integer $i$. 
For example, if there are two calls to $\SolidityNonDetFn$ in $\phi$, then we get $\phi_0$ by replacing the calls with $\{\bfalse,\bfalse\}$; similarly, we get $\phi_2$ by replacing calls with $\{\btrue,\bfalse\}$ respectively. 
\item Convert $\phi$ to a negation-normal form $\hat{\phi}$ where a call to $\SolidityNonDetFn{}$ either appears negatively or positively.
Next, we replace any negative (respectively, positive) occurrence of the call with $\bfalse$ (respectively, $\btrue$). 
\end{enumerate}
The first check is sound but overly conservative as it will fail many \texttt{require} that mention a global role.
For runtime checking it is undesirable to revert transactions conservatively in the absence of information about global roles. 
Since global roles are already being checked by Workbench, we would like to revert a transaction only when we are guaranteed that it fails the specification. 
In contrast, the second check weakens the predicate $\phi$ and therefore a failure will be a true violation of the intended specification we outlined in Section~\ref{sec:semantic-conformance}.
In essence, the second transformation replaces calls to the non-deterministic function in \texttt{require} (respectively, \texttt{assert}) with $\btrue$ (respectively, $\bfalse$).
We therefore use the second transformation of $\phi$ for installing runtime checks. 

Figure~\ref{fig:instrumented-running-example-runtime} describes the actual checks that are inserted for runtime enforcement using the second transformation described above. 
We show the original expressions in comments.
As noted, the (positive) occurrence of $\SolidityNonDetFn$ in $\solRequire$ statements are replaced with $\btrue$ making the $\solRequire$ in \texttt{constructor\_checker} true.
The (negative) occurrence of $\SolidityNonDetFn$ in \texttt{SendResponse\_checker} is replaced with $\bfalse$ making the $\solAssert$ true. 
Therefore, for this example, we only check two assertions related to initial state and state transition when invoking \texttt{SendRequest}. 

\begin{figure}[htbp]
\begin{lstlisting}[style=Sol,numbers=none]
    // Checker modifiers 
    modifier constructor_checker() 
    {
      // require (msg.sender != tx.origin || 
      //          NonDetFunc()); 
      require (true); 
       _;      
      assert (State == StateType.Request);
    }
    modifier SendRequest_checker() 
    {
      StateType oldState = State;
      address oldRequestor = Requestor;
       _;
      assert ((msg.sender == oldRequestor && 
               oldState == StateType.Respond) 
              ==> State == StateType.Request);
    }
    modifier SendResponse_checker() 
    {
      StateType oldState = State;
       _;
      //assert ((NonDetFunc() && 
      //         oldState == StateType.Request) 
      //         ==> State == StateType.Respond);
      assert (true);
    }

\end{lstlisting}
\vspace{-0.1in}
\caption{Modifier definitions for instrumented HelloBlockchain application for runtime checking.}
\label{fig:instrumented-running-example-runtime}
\end{figure}

\section{Semantics for Assignments}

\begin{figure}[htbp]
\centering
\includegraphics[scale=0.7]{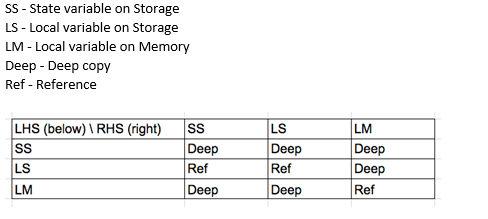}
\vspace{-0.1in}
\caption{Semantics of Solidity array assignment LHS = RHS.}
\label{fig:sol-arr-semantics}
\end{figure}
  
\end{appendix}
